# Supplementary material for: Predicting Causes of Reformulation in Intelligent Assistants
Source: arXiv:1707.03968 source file (2017-07-13)
Supplement: Supplementary file 1 [file appendix.tex]

% \section{Complete List of Features}
% Table \ref{tab:feature} is the complete list of features. \\
% \begin{table*}[t]
%   \begin{center}
%  %   \footnotesize
%     \begin{tabular}{lll}
%       \textbf{Category} & \textbf{Name} & \textbf{Definition}\\ \hline
%       %%%%%
%       Session & \textbf{CharLen*} & Number of characters \\
%       & \textbf{WordLen*} & Number of words \\
%       & \textbf{Interval} & Time between $U_1$ and $U_2$ \\
%       & \textbf{Voice2Text} & 1 if $U_1$ is voice input and $U_2$ is text input \\ \hdashline
%       Similarity & \textbf{EditDistance} & Normalized Levenshtein edit distance between $U_1$ and $U_2$ \\
%       & \textbf{Generarization} & 1 if $U_2$ is a generarization of $U_1$ \\
%       & \textbf{Specification} & 1 if $U_2$ is a specification of $U_1$ \\ \hdashline
%       % & \textbf{Reformulation($p$)} & 1 if $U_2$ matches reformulation pattern $p$ of $U_1$ \\
%       % & \textbf{CommonWordsU} & Number of words both in $U_1$ and $U_2$ \\
%       % & \textbf{CommonWordsR} & Number of words both in $R$ and $U_2$ \\ \hdashline
%       IA specific & \textbf{SameFunction} & 1 if response functions beweeen $U_1$ and $U_2$ are same \\
%       & \textbf{DifferentFunction} & 1 if response functions beweeen $U_1$ and $U_2$ are different \\
%       & \textbf{DifferentSlot} & 1 if some slots in $U_2$ is different from that in $U_1$ \\
%       & \textbf{Positive*} & 1 if the utterance contains positive phrases \\
%       & \textbf{Negative*} & 1 if the utterance contains negative phrases \\ \hdashline
%       % & \textbf{Positive($c$)*} & 1 if the utterance contains positive phrases of category $c$ \\
%       % & \textbf{Negative($c$)*} & 1 if the utterance contains negative phrases of category $c$ \\ \hdashline
%       Speech & \textbf{SRConf*} & Speech recognition confidence \\
%       & \textbf{VoiceLen*} & Speech recognition time \\
%       %%%%%%%
%       %%%%%%%%
%     \end{tabular}
%     \caption{List of features. Features marked with an ``*'' were computed for both $U_1$ and $U_2$.}
%     \label{tab:feature}
%   \end{center}
% \end{table*}
